# Supplementary material for: Tetrahedrality dictates dynamics in hard spheres
Source: arXiv:1908.00425 ancillary file (2019-08-01)
Supplement: Supplementary file 1 [file SI.pdf]

# Tetrahedrality dictates dynamics in hard spheres: Supplemental Information

Susana Marín-Aguilar, Henricus H. Wensink, Giuseppe Foffi, and Frank Smallenburg
*Laboratoire de Physique des Solides, CNRS, Université Paris-Sud, Université Paris-Saclay, 91405 Orsay, France*

## CLUSTERS CORRELATED WITH ICOSAHEDRAL ORDER

As shown in the main text, the fraction of particles involved in an icosahedral cluster correlates significantly with the diffusivity of different binary systems at constant packing fraction $\eta = 0.575$. However, there are a number of other clusters which can be detected using the Topological Cluster Classification algorithm [1] which correlate strongly with the appearance of icosahedral clusters. To illustrate this, we show in Fig. S1 the fraction of particles involved in a variety of clusters, as a function of the composition. Each of the clusters displayed here contains a ring of five particles, and hence partially captures the five-fold symmetry of the full icosahedral cluster. As Fig. S1 shows, the prevalence of each of the chosen clusters shows approximately the same behavior, making it difficult to identify any one of them as mainly responsible for slow dynamics.

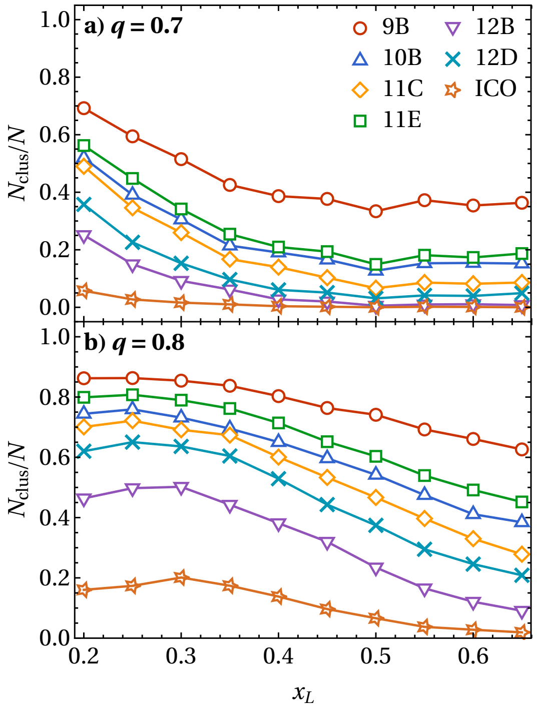


FIG. S1: Fraction of particles $N_{\rm clus}/N$ involved in different local clusters as indicated, for binary systems with fixed packing fraction $\eta = 0.575$ and size ratio $q = 0.7$ (a) and 0.8 (b). Note that ICO corresponds to a full icosahedral cluster.

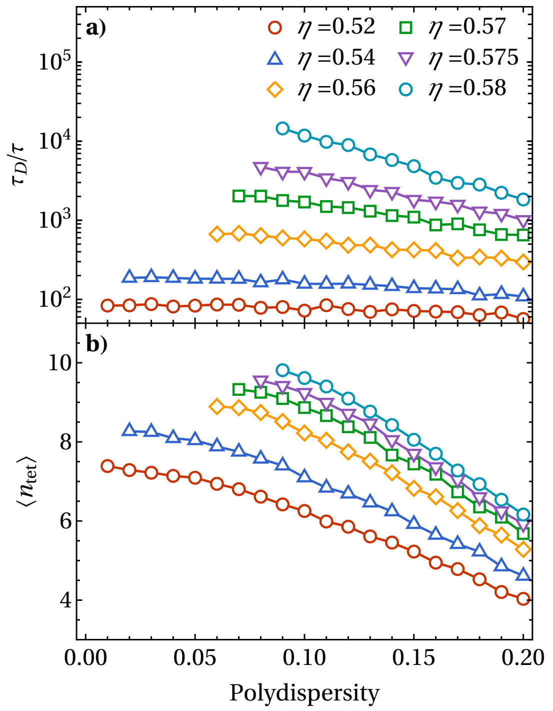


FIG. S2: a) Average tetrahedrality $\langle n_{\rm tet}\rangle$ as a function of polydispersity for polydisperse hard-sphere mixtures. b) Diffusion time $\tau_D$ for the same systems. $\tau$ is the time unit of the simulations. The polydispersity is defined as the standard deviation of the particle diameters, normalized by the average diameter.

## TETRAHEDRALITY AND MOBILITY OF POLYDISPERSE SYSTEMS

In Fig. S2, we plot the average tetrahedrality $\langle n_{\rm tet}\rangle$ and diffusion time $\tau_D$ as a function of the polydispersity for all investigated polydisperse systems. As with the binary systems, the influence of tetrahedrality increases with increasing packing fraction.

## CORRELATION BETWEEN LOCAL TETRAHEDRALITY AND LOCAL MOBILITY

In the main text, we focus on the correlations between local tetrahedrality and local mobility in one of our slowest binary systems, with packing fraction $\eta = 0.575$, size ratio $q = 0.8$, and composition $x_L = 0.3$. Here, we provide results for some faster systems, in order to illustrate the strength of the correlations in systems where the dy-

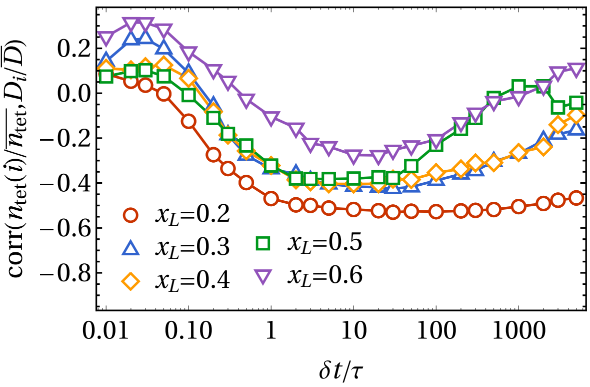


FIG. S3: Rank correlation between the number of tetrahedra for a particle $n_{\rm tet}$ and the dynamic propensity $D_i$ for several binary systems with size ratio $q = 0.75$, packing fraction $\eta = 0.575$, and various compositions $x_L$ as indicated. Only results for the small particles are shown. The large particles show similar behavior.

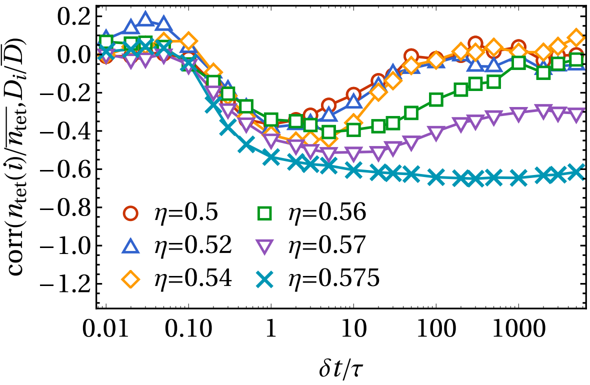


FIG. S4: Rank correlation between the number of tetrahedra for a particle $n_{\rm tet}$ and the dynamic propensity $D_i$ for several binary systems with size ratio $q = 0.8$, composition $x_L = 0.3$, and various packing fractions $\eta$ as indicated. Only results for the small particles are shown. The large particles show similar behavior.

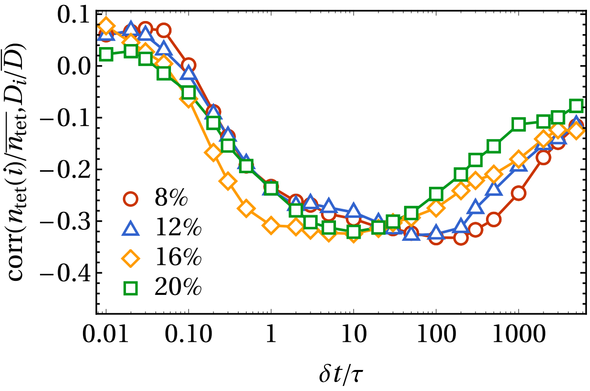


FIG. S5: Rank correlation between the number of tetrahedra for a particle $n_{\rm tet}$ and the dynamic propensity $D_i$ for several polydisperse systems at packing fraction $\eta = 0.575$. Different colors denote different polydispersities as indicated.

namics are less heterogeneous. For each system, we show the Spearman's rank correlation between the number of tetrahedra for a given particle $n_{\rm tet}(i)$ and its dynamic propensity $D_i$, averaged over 100 runs starting from the same initial snapshot.

In Fig. S3, we show correlations for several binary systems at a fixed high packing fraction $\eta = 0.575$ and a fixed size ratio $q = 0.75$. As Fig. 1 in the main text shows, for these systems the diffusion time $\tau_D$ gradually decrases as the composition increases. Indeed, S5 shows a shift of the minimum in the correlation to shorter times as $x_L$ increases from 0.2 to 0.6. This shift is accompanied by a decrease in overall correlation strength, which can be attributed the weaker overall heterogeneity in the dynamics we observe in these systems.

In Fig. S4, we show the same correlations for binary systems at a the composition and size ratio of our slowest system ($q = 0.8$, $x_L = 0.3$), with varying packing fractions. Again, as the we move to faster systems (lower packing fractions), we observe a decrease in the overall predictiveness of the tetrahedrality, as well as a shift to shorter time scales. Nonetheless, strong correlations are observed in the full range of explored packing fractions.

Figure S5 shows correlations for several polydisperse systems. Note that we here consider all particle sizes in our calculation. Naturally, this leads to an inherent negative correlation, as larger particles tend to both be involved in more tetrahedra and have lower mobility. To correct for this, before calculating the correlation, we normalize the dynamic propensity $D_i$ of each particle with the average $\overline{D}$ for all particles of its size, and similarly normalize $n_{\rm tet}(i)$ by dividing by the associated $\overline{n_{\rm tet}}$. As the polydispersity increases, the minimum in the correlation shifts to shorter times. This is consistent with the overall faster dynamics of systems with higher polydispersity shown in Fig. S2. Interestingly, the strength of the correlation is not significantly affected by the change in polydispersity. In Fig. S6, we show snapshots for the slowest of these polydisperse systems, with particles colored according to their tetrahedrality $n_{\rm tet}(i)$, displacement $\delta r_i$ after a time interval $\delta t = 100\tau$, and dynamic propensity after the same time interval. As the correlations in Fig. S5 indicate, we again see strong correlations between tetrahedrality and the mobility of the particles.

[1] A. Malins, J. Eggers, C. P. Royall, S. R. Williams, and H. Tanaka, J. Chem. Phys. **138**, 12A535 (2013).

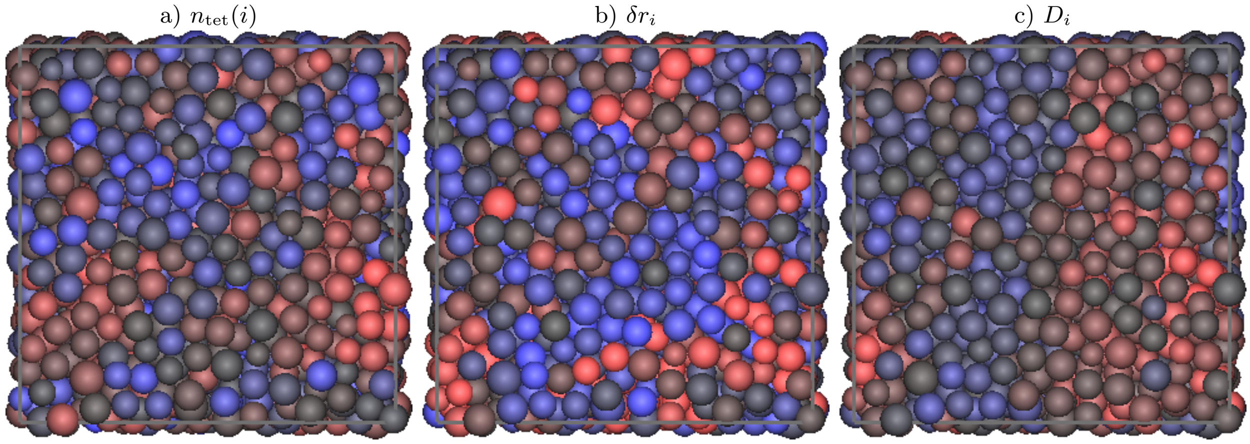


FIG. S6: Snapshots of a glassy polydisperse system (packing fraction $\eta = 0.575$, polydispersity 8%, with particles colored according to different criteria. a) According to the number of tetrahedra $n_{\mathrm{tet}}(i)$ a particle is involved in, with red particles involved in fewer tetrahedra, and blue particles in more. b) According to the absolute displacement $\delta r_i$ after a time interval $\delta t = 100\tau$ in a random trajectory, with red indicating fast particles and blue indicating slow ones. c) According to the dynamic propensity $D_i$ over the same time interval. In all snapshots, the color gray indicates the average for each of the 15 distinct particle sizes.
